# Supplementary material for: ADEPT: Hierarchical Bayes Approach to Personalized Federated Unsupervised Learning
Source: arXiv:2402.12537 source file (2025-01-24)
Supplement: Supplementary file 2 [file appendix_related_works.tex]

%As mentioned earlier, there has been several recent works on personalized \emph{supervised} learning, and we give a more detailed accounting of it in Appendix \ref{app:RelWrk}. There has been much less attention given to personalized federated unsupervised learning. The closest work to ours on personalized dimensionality reduction are \cite{shi2022personalized,ozkara2023isit} which study personalized PCA algorithms. \cite{shi2022personalized} has a restrictive assumption that principal components for global and local models are non-overlapping. \cite{ozkara2023isit} uses the hierarchical Bayes statistal model to develop a criterion for personalized PCA; however, the authors assume heterogeneity of the setting is known; in contrast, \texttt{ADEPT-PCA} learns and adapts the solution accordingly. There is some literature on on specific tasks such as training recommender systems \citep{le2022personalized,Mirko2021}, grouping clients based on latent representations \citep{yang2023personalized}, generating data to improve performance of personalized supervised learning \cite{Cao2023, peng2023}. However, our approach to develop personalized dimensionality reduction for heterogeneous data is quite distinct from them. We are not aware of any FL work for personalized diffusion generative models. There is work using pre-trained diffusion models and then fine-tuning them \citep{ruiz2023dreambooth, zhang2023adding, moon2022fine, ma2023subject}. However, these do not fit into the federated learning paradigm, and require data collection from clients to obtain the pre-trained model. One way to view our approach, is to \emph{simultaneously} build such ``global'' models (akin to pre-trained models) and individual (personalized) models, while not sharing data.

%As mentioned earlier, there has been several recent works on personalized \emph{supervised} learning, and we give a more detailed accounting of it in Appendix \ref{app:RelWrk}. There has been much less attention given to personalized federated unsupervised learning. The closest work to ours on personalized dimensionality reduction are \cite{shi2022personalized,ozkara2023isit} which study personalized PCA algorithms. \cite{shi2022personalized} has a restrictive assumption that principal components for global and local models are non-overlapping. \cite{ozkara2023isit} uses the hierarchical Bayes statistal model to develop a criterion for personalized PCA; however, the authors assume heterogeneity of the setting is known, whereas, our PCA method learns it during training and adapts the problem accordingly. Therefore the algorithm in  \cite{ozkara2023isit} does not learn the adaptation to balance local data and collaboration and is tailored to linear dimensionality reduction. There is some literature on on specific tasks such as training recommender systems \citep{le2022personalized,Mirko2021}, grouping clients based on latent representations \citep{yang2023personalized}, generating data to improve performance of personalized supervised learning \cite{Cao2023, peng2023}. However, our approach to develop personalized dimensionality reduction for heterogeneous data is quite distinct from them.

%We are not aware of any personalized FL work for training diffusion models. The closest work is \citep{tun2023federated} where the authors investigate local features of globally trained models through FedAvg, but do not build personalized generative models. There is a much larger line of work on using pre-trained diffusion models and then personalizing/fine-tuning them \citep{ruiz2023dreambooth, zhang2023adding, moon2022fine, ma2023subject}. However, these do not fit into the federated learning paradigm, and require data collection from clients to obtain the pre-trained model. One way to view our approach, is to \emph{simultaneously} build such ``global'' models (akin to pre-trained models) and individual (personalized) models, while not sharing data.




%\textbf{Personalized FL. } 

%\citep{ozkara2022statistical}

%\textbf{Personalized unsupervised FL. }
%Personalized unsupervised FL (PUFL) received much less attention. Recent work in literature combined unsupervised algorithms with personalized FL (as a means rather than end goal) for specific tasks such as training recommender systems \citep{le2022personalized,Mirko2021}, grouping clients based on latent representations \citep{yang2023personalized}, generating data to improve performance of personalized supervised learning \cite{Cao2023, peng2023}. We have come across only a few fundamental research in personalized unsupervised FL where the goal is to reveal insights about clients' distinct underlying data distributions through collaboration. To that end, \cite{shi2022personalized,ozkara2023isit} proposes personalized PCA algorithms. \cite{shi2022personalized} has a restrictive assumption that principal components for global and local models are non-overlapping. Similar to us \cite{ozkara2023isit} uses \cite{ozkara2023a} to formulate the problem; however, the authors assume heterogeneity of the setting is known; in contrast, \texttt{ADEPT-PCA} learns and adapts the solution accordingly. We are not aware of any personalized FL work for training diffusion models. The closest work is \citep{tun2023federated} where the authors investigate local features of globally trained models through FedAvg. Outside of the context of FL, personalizing/fine-tuning pre-trained diffusion models received much more attention \citep{ruiz2023dreambooth, zhang2023adding, moon2022fine, ma2023subject}. However, these do not fit into the federated learning paradigm, and require data collection from clients to obtain the pre-trained model. One way to view our approach, is to \emph{simultaneously} build such ``global'' models (akin to pre-trained models) and individual (personalized) models, while not sharing data.
